# Supplementary material for: XTREME-UP: A User-Centric Scarce-Data Benchmark for Under-Represented Languages
Source: arXiv:2305.11938 source file (2023-05-24)
Supplement: Supplementary file 1 [file appendix_retrieval_for_qa.tex]

\subsection{Retrieval for Question Answering (QA)} \label{app:qa-retrieval}
